# Supplementary material for: Valence Transition Theory of the Pressure-Induced Dimensionality Crossover in Superconducting Sr$_{14-x}$Ca$_x$Cu$_{24}$O$_{41}$
Source: arXiv:2207.00628 ancillary file (2023-10-12)
Supplement: Supplementary file 1 [file supplemental.pdf]

# Valence Transition Theory of the Pressure-Induced Dimensionality Crossover in Superconducting $\text{Sr}_{14-x}\text{Ca}_x\text{Cu}_2\text{O}_{41}$

Jeong-Pil Song,<sup>1</sup> R. Torsten Clay,<sup>2</sup> and S. Mazumdar<sup>1</sup>

<sup>1</sup>*Department of Physics, University of Arizona, Tucson, AZ 85721*

<sup>2</sup>*Department of Physics and Astronomy and HPC<sup>2</sup> Center for Computational Sciences, Mississippi State, MS 39762*

(Dated: June 15, 2022)

## S.1. DENSITY MATRIX RENORMALIZATION GROUP METHOD

In this work, we carried out the DMRG calculations using our DMRG code with the Itensor library [S1,2]. The calculations were performed using conserved particle number and the  $z$  component of the total spin ( $S_z$ ) for increasing values of the bond dimension  $m$ . In order to avoid getting stuck into local minima we added noise with a large number of sweeps for small values of bond dimension  $m$ . The calculations for various different types of bond orders, charge densities, and total energies were carried out using the bond dimension of up to  $m = 13000$ . We have excluded any results for the small value of  $m$  ( $< 5000$ ) to systematically remove uncontrolled errors and computational artifacts from the lack of parameter space. We found that for each parameter set fully converged bond orders can be obtained with the bond dimension  $m$  of 6400–13000 up to 116 sites ( $12 \times 2$ -rung) by performing linear extrapolations in the limit of zero truncation error. Furthermore, in order to achieve a precise estimate for the DMRG energies with open boundary conditions, the maximal bond dimension  $m$  of 13000 up to 156 sites ( $16 \times 2$ -rung) we used is also sufficient to extrapolate spin gaps in the infinite ladder length limit ( $L \rightarrow \infty$ ). Note that a unit length is defined by the distance between two parallel Cu-O-Cu rungs along the leg direction.

## S.2. SPIN GAPS

In Fig. S1 we show a typical DMRG extrapolation of the total energies as a function of the DMRG truncation error for  $S_z = 0$  and  $S_z = 1$  on a  $16 \times 2$ -rung multiorbital ladder. In each case we first used the standard DMRG linear extrapolation using the three smallest truncation error points in order to estimate the extrapolated value to the infinite bond dimension limit (corresponding to the zero DMRG truncation error). We then performed a finite-size scaling analysis of the spin gap  $\Delta_s$  against inverse ladder length  $1/L$ . In all cases we used the ladder lengths of up to 16. Finally, we estimated the spin gap in the thermodynamic limit using a quadratic fit in  $1/L$ . Fig. S2 shows the finite-size scaling of the  $\Delta_s$  in the undoped ( $\delta = 0$ ) ladder model. For comparison, in Fig. S2(a) we also provide the  $\Delta_s$  for single ladders. For both single (Fig. S2(a)) and coupled (Fig. S2(b)) multiorbital ladders, we found that a quadratic fit in  $1/L$  performs well.

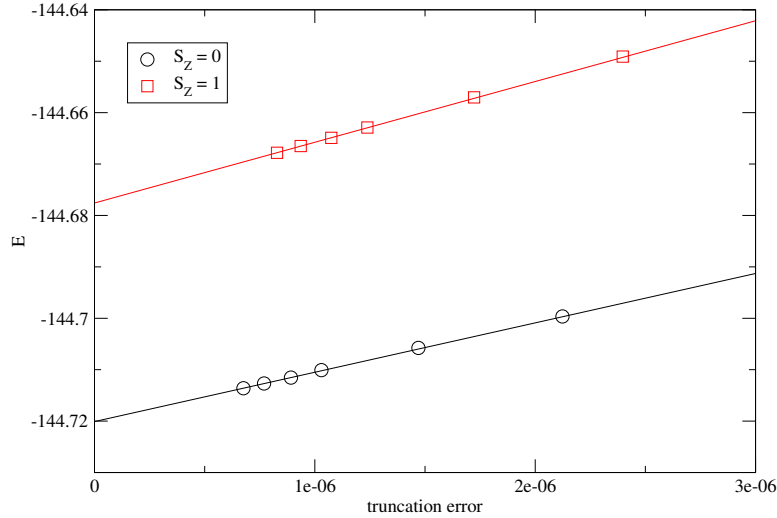

FIG. S1: DMRG extrapolations of total energies as a function of DMRG truncation error in the undoped ( $\delta = 0$ ) coupled ladder model for a  $16 \times 2$ -rung multiorbital ladder with  $U_d = 8$ ,  $U_p = 3$ ,  $t_{pp} = 0.5$ ,  $t'_{pp} = 0.5$ ,  $t_{dp} = 1$  and  $\Delta_{dp} = 2$ . In each case, the extrapolated value to the infinite bond dimension limit ( $m \rightarrow \infty$ ) was estimated from a linear fit using the three smallest truncation error points. Circles and squares are for  $S_z = 0$  and  $S_z = 1$ , respectively. The lines are linear fits.

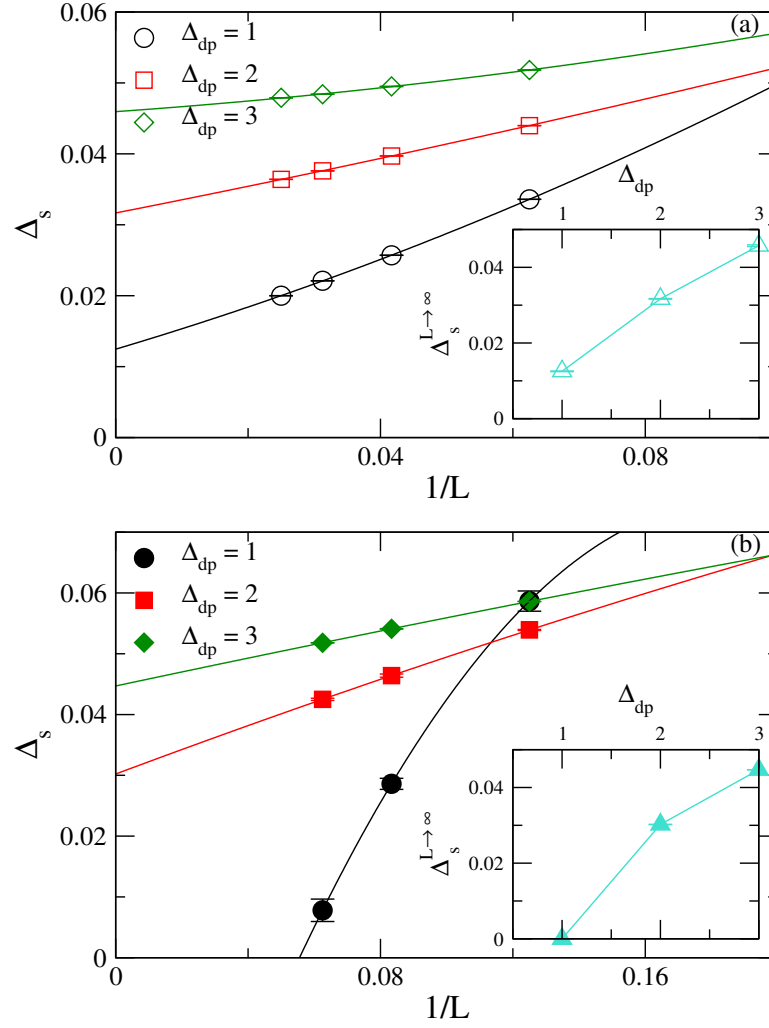

FIG. S2: Finite size extrapolation of the spin gap  $\Delta_s$  in the undoped ( $\delta = 0$ ) ladder with  $U_d = 8$ ,  $U_p = 3$ ,  $t_{pp} = 0.5$ ,  $t'_{pp} = 0.5$ , and  $t_{dp} = 1$ . (a) Single and (b) coupled ladders. The lines are quadratic fits. Insets show the extrapolated spin gap  $\Delta_s^{L \rightarrow \infty}$  as a function of  $\Delta_{dp}$ .

### S.3. BOND ORDERS

In Fig. S3 we show a typical DMRG extrapolation of the average bond orders as a function of the DMRG truncation error. Note that we here took an average over the bond order terms that are not connected to the outer boundary sites in order to alleviate boundary effects as a consequence of Friedel oscillations in the open boundary DMRG. Table I further summarizes our extrapolated DMRG results for the bond orders. In fig. S4 we present a finite-size scaling analysis of the bond orders in the noninteracting ( $U_d = U_p = 0$ ) multiband coupled ladder. In Table II we further provide a list of bond orders for the noninteracting ladders for  $\delta = 0.125$ .

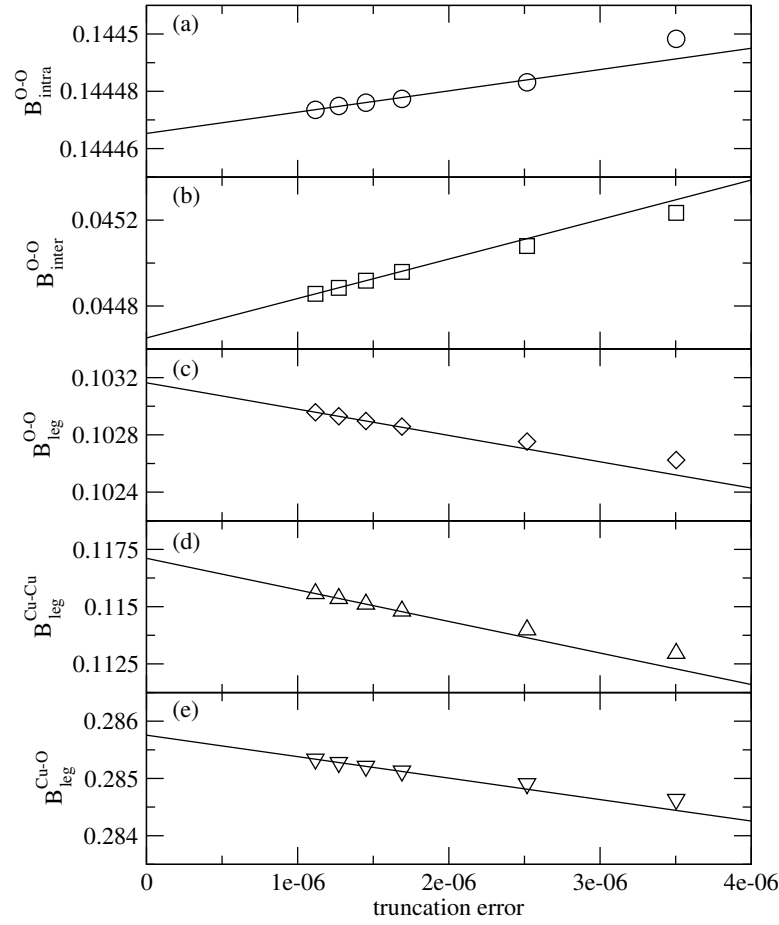

FIG. S3: DMRG extrapolations of average bond orders as a function of DMRG truncation error in the weakly doped ( $\delta = 0.0625$ ) coupled ladder model with  $U_d = 8$ ,  $U_p = 3$ ,  $t_{pp} = 0.5$ ,  $t'_{pp} = 0.5$ ,  $t_{dp} = 1$  and  $\Delta_{dp} = 3$  for a  $8 \times 2$ -rung multiorbital ladder. In each case, the extrapolated value to the infinite bond dimension limit ( $m \rightarrow \infty$ ) was obtained from a linear fit using the three smallest truncation error points. Circles, squares, diamonds, up triangles, and down triangles correspond to (a)  $B_{\text{intra}}^{\text{O-O}}$ , (b)  $B_{\text{inter}}^{\text{O-O}}$ , (c)  $B_{\text{leg}}^{\text{O-O}}$ , (d)  $B_{\text{leg}}^{\text{Cu-Cu}}$ , and (e)  $B_{\text{leg}}^{\text{Cu-O}}$ , respectively. The lines are linear fits.

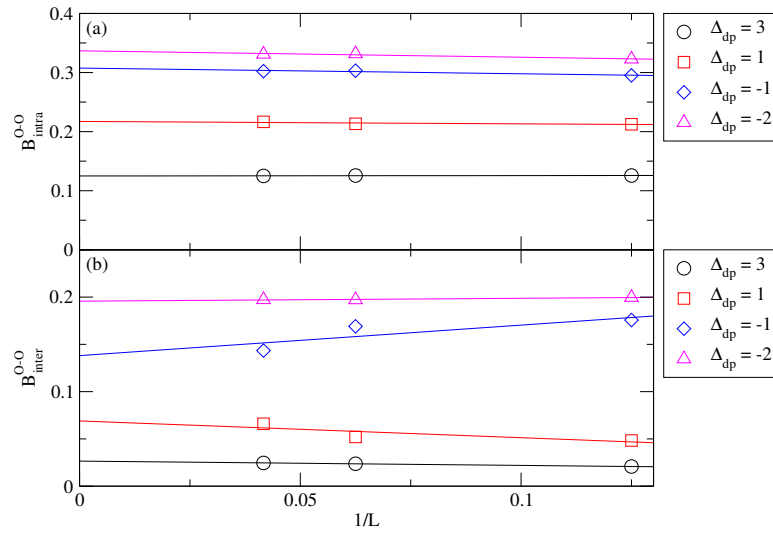

FIG. S4: Size dependence of bond orders for  $\delta = 0.125$  and  $t'_{pp} = 0.5$  in the noninteracting ( $U_d = U_p = 0$ ) multiband coupled ladder with  $t_{pp} = 0.5$  and  $t_{dp} = 1$ , with periodic boundary condition, along the ladder leg and rung directions. (a)  $B_{\text{intra}}^{\text{O-O}}$  and (b)  $B_{\text{inter}}^{\text{O-O}}$ . The lines are linear fits.

TABLE I: Extrapolated average bond orders in the multiband  $8 \times 2$  and  $12 \times 2$  coupled ladders for  $U_d = 8$ ,  $U_p = 3$ ,  $t_{pp} = 0.5$ , and  $t_{dp} = 1$ . All results are extrapolated to the zero truncation limit. In all cases, the error bars of the DMRG bond orders are  $\sim O(10^{-4})$  or smaller.

| $L$ | $t'_{pp}$ | $\delta$ | $\Delta_{dp}$ | $B_{\text{intra}}^{\text{O-O}}$ | $B_{\text{inter}}^{\text{O-O}}$ | $B_{\text{leg}}^{\text{O-O}}$ | $B_{\text{leg}}^{\text{Cu-Cu}}$ | $B_{\text{leg}}^{\text{Cu-O}}$ |
|-----|-----------|----------|---------------|---------------------------------|---------------------------------|-------------------------------|---------------------------------|--------------------------------|
| 8   | 0.3       | 0.0625   | 3             | 0.1417                          | 0.0258                          | 0.1039                        | 0.1137                          | 0.2804                         |
| 8   | 0.3       | 0.125    | 3             | 0.1657                          | 0.0250                          | 0.1260                        | 0.1319                          | 0.3075                         |
| 8   | 0.3       | 0.1875   | 3             | 0.1834                          | 0.0293                          | 0.1337                        | 0.1250                          | 0.3228                         |
| 8   | 0.3       | 0.25     | 3             | 0.1945                          | 0.0329                          | 0.1363                        | 0.1260                          | 0.3395                         |
| 8   | 0.5       | 0.0625   | 3             | 0.1445                          | 0.0447                          | 0.1032                        | 0.1171                          | 0.2858                         |
| 8   | 0.5       | 0.125    | 3             | 0.1678                          | 0.0461                          | 0.1227                        | 0.1311                          | 0.3105                         |
| 8   | 0.5       | 0.1875   | 3             | 0.1850                          | 0.0579                          | 0.1297                        | 0.1185                          | 0.3249                         |
| 8   | 0.5       | 0.25     | 3             | 0.1958                          | 0.0585                          | 0.1294                        | 0.1276                          | 0.3421                         |
| 12  | 0.3       | 0.125    | 3             | 0.1584                          | 0.0255                          | 0.1170                        | 0.1240                          | 0.2993                         |
| 12  | 0.3       | 0.125    | 2             | 0.1943                          | 0.0371                          | 0.1472                        | 0.1552                          | 0.3328                         |
| 12  | 0.3       | 0.125    | 1             | 0.2340                          | 0.0536                          | 0.1789                        | 0.1693                          | 0.3540                         |
| 12  | 0.3       | 0.125    | -1            | 0.2945                          | 0.0990                          | 0.2256                        | 0.1366                          | 0.3432                         |
| 12  | 0.3       | 0.125    | -2            | 0.3147                          | 0.1156                          | 0.2291                        | 0.1071                          | 0.3133                         |
| 12  | 0.5       | 0.125    | 3             | 0.1629                          | 0.0475                          | 0.1169                        | 0.1314                          | 0.3077                         |
| 12  | 0.5       | 0.125    | 2             | 0.1961                          | 0.0645                          | 0.1402                        | 0.1536                          | 0.3343                         |
| 12  | 0.5       | 0.125    | 1             | 0.2338                          | 0.0964                          | 0.1598                        | 0.1637                          | 0.3536                         |
| 12  | 0.5       | 0.125    | -1            | 0.2901                          | 0.1570                          | 0.1961                        | 0.1366                          | 0.3408                         |
| 12  | 0.5       | 0.125    | -2            | 0.3056                          | 0.2189                          | 0.1530                        | 0.1010                          | 0.2999                         |

TABLE II: Bond orders for  $\delta = 0.125$  in the noninteracting ( $U_d = U_p = 0$ ) multiband  $L \times 2$  coupled ladder with  $t_{pp} = 0.5$  and  $t_{dp} = 1$ , with periodic boundary condition, along the ladder leg and rung directions.

| $L$ | $t'_{pp}$ | $\Delta_{dp}$ | $B_{\text{intra}}^{\text{O-O}}$ | $B_{\text{inter}}^{\text{O-O}}$ | $B_{\text{leg}}^{\text{O-O}}$ | $B_{\text{leg}}^{\text{Cu-Cu}}$ | $B_{\text{leg}}^{\text{Cu-O}}$ |
|-----|-----------|---------------|---------------------------------|---------------------------------|-------------------------------|---------------------------------|--------------------------------|
| 8   | 0.3       | 3             | 0.1241                          | 0.0147                          | 0.1101                        | 0.3749                          | 0.3350                         |
| 8   | 0.3       | 2             | 0.1647                          | 0.0227                          | 0.1451                        | 0.3320                          | 0.3651                         |
| 8   | 0.3       | 1             | 0.2113                          | 0.0340                          | 0.1872                        | 0.2817                          | 0.3833                         |
| 8   | 0.3       | -1            | 0.3163                          | 0.0682                          | 0.2069                        | 0.1125                          | 0.3151                         |
| 8   | 0.3       | -2            | 0.3484                          | 0.0796                          | 0.2293                        | 0.0874                          | 0.2848                         |
| 16  | 0.3       | 3             | 0.1251                          | 0.0175                          | 0.1085                        | 0.3727                          | 0.3357                         |
| 16  | 0.3       | 2             | 0.1659                          | 0.0264                          | 0.1433                        | 0.3294                          | 0.3658                         |
| 16  | 0.3       | 1             | 0.2128                          | 0.0386                          | 0.1857                        | 0.2781                          | 0.3836                         |
| 16  | 0.3       | -1            | 0.3080                          | 0.0694                          | 0.2407                        | 0.1395                          | 0.3365                         |
| 16  | 0.3       | -2            | 0.3390                          | 0.0800                          | 0.2695                        | 0.1055                          | 0.3042                         |
| 24  | 0.3       | 3             | 0.1269                          | 0.0122                          | 0.1045                        | 0.3364                          | 0.3256                         |
| 24  | 0.3       | 2             | 0.1686                          | 0.0182                          | 0.1376                        | 0.2968                          | 0.3542                         |
| 24  | 0.3       | 1             | 0.2167                          | 0.0262                          | 0.1774                        | 0.2509                          | 0.3707                         |
| 24  | 0.3       | -1            | 0.3105                          | 0.0902                          | 0.2166                        | 0.1244                          | 0.3265                         |
| 24  | 0.3       | -2            | 0.3418                          | 0.1059                          | 0.2397                        | 0.0953                          | 0.2947                         |
| 8   | 0.5       | 3             | 0.1250                          | 0.0208                          | 0.1090                        | 0.3759                          | 0.3363                         |
| 8   | 0.5       | 2             | 0.1659                          | 0.0323                          | 0.1427                        | 0.3339                          | 0.3665                         |
| 8   | 0.5       | 1             | 0.2125                          | 0.0483                          | 0.1826                        | 0.2847                          | 0.3842                         |
| 8   | 0.5       | -1            | 0.2952                          | 0.1757                          | 0.2150                        | 0.1412                          | 0.3411                         |
| 8   | 0.5       | -2            | 0.3228                          | 0.1996                          | 0.2387                        | 0.1066                          | 0.3057                         |
| 16  | 0.5       | 3             | 0.1257                          | 0.0237                          | 0.1082                        | 0.3728                          | 0.3372                         |
| 16  | 0.5       | 2             | 0.1666                          | 0.0359                          | 0.1425                        | 0.3299                          | 0.3672                         |
| 16  | 0.5       | 1             | 0.2133                          | 0.0521                          | 0.1838                        | 0.2791                          | 0.3842                         |
| 16  | 0.5       | -1            | 0.3032                          | 0.1691                          | 0.1817                        | 0.1193                          | 0.3221                         |
| 16  | 0.5       | -2            | 0.3317                          | 0.1971                          | 0.1959                        | 0.0925                          | 0.2885                         |
| 24  | 0.5       | 3             | 0.1257                          | 0.0246                          | 0.1077                        | 0.3694                          | 0.3369                         |
| 24  | 0.5       | 2             | 0.1666                          | 0.0370                          | 0.1421                        | 0.3263                          | 0.3668                         |
| 24  | 0.5       | 1             | 0.2166                          | 0.0660                          | 0.1673                        | 0.2360                          | 0.3690                         |
| 24  | 0.5       | -1            | 0.3023                          | 0.1434                          | 0.2143                        | 0.1349                          | 0.3338                         |
| 24  | 0.5       | -2            | 0.3310                          | 0.1973                          | 0.1988                        | 0.0896                          | 0.2895                         |

#### S.4. CHARGE DENSITIES

In Fig. S5 we show a typical DMRG extrapolation of the average charge densities  $\langle n_{Cu} \rangle$ ,  $\langle n_{O_R} \rangle$ , and  $\langle n_{O_L} \rangle$  as a function of the DMRG truncation error. Note that here we took the average over all Cu,  $O_R$  and  $O_L$  sites on the coupled ladder to preserve charge conservation. Table III fully summarizes our extrapolated DMRG results for the charge densities. For comparison, in Table IV we also provide a list of charge densities for the noninteracting ladders for  $\delta = 0.125$ .

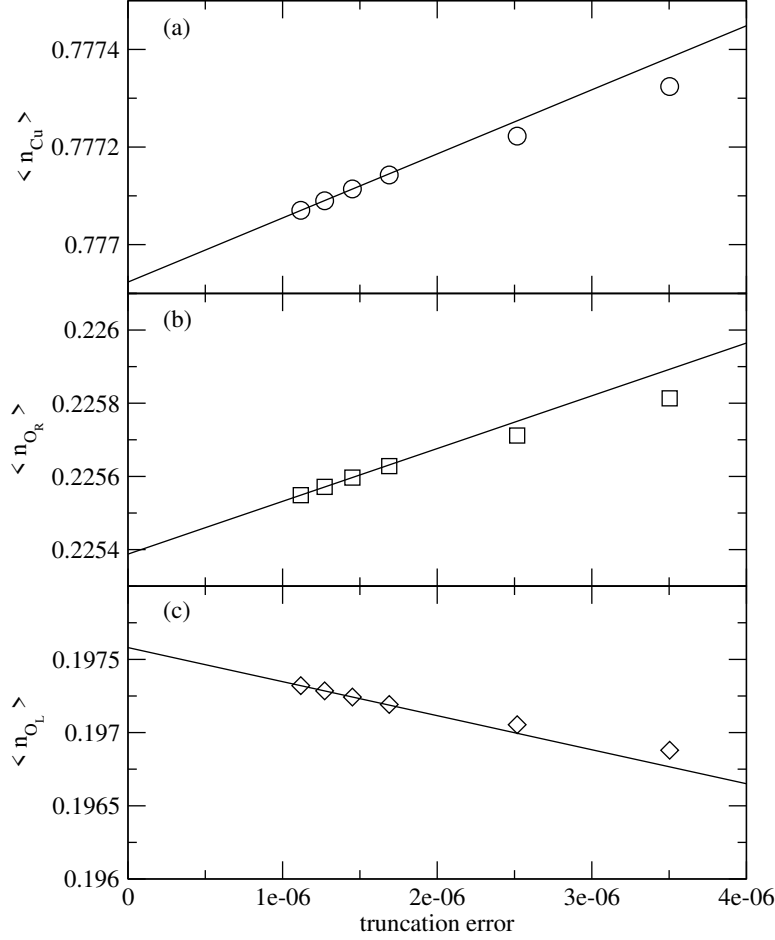

FIG. S5: DMRG extrapolations of average charge densities as a function of DMRG truncation error for the same parameters as in Fig. S3. The lines are linear fits.

TABLE III: Extrapolated average charge densities on Cu and O sites in the coupled  $L \times 2$  ladder with  $U_d = 8$ ,  $U_p = 3$ ,  $t_{pp} = 0.5$ , and  $t_{dp} = 1$ . All results are extrapolated to the zero truncation limit. In all cases, the error bars on the DMRG charge densities are  $\sim O(10^{-4})$  or smaller.

| $L$ | $t'_{pp}$ | $\delta$ | $\Delta_{dp}$ | $\langle n_{Cu} \rangle$ | $\langle n_{O_R} \rangle$ | $\langle n_{O_L} \rangle$ |
|-----|-----------|----------|---------------|--------------------------|---------------------------|---------------------------|
| 8   | 0.3       | 0        | 3             | 0.7636                   | 0.1975                    | 0.1574                    |
| 8   | 0.3       | 0.0625   | 3             | 0.7791                   | 0.2277                    | 0.1938                    |
| 8   | 0.3       | 0.125    | 3             | 0.7943                   | 0.2594                    | 0.2298                    |
| 8   | 0.3       | 0.1875   | 3             | 0.8129                   | 0.2933                    | 0.2605                    |
| 8   | 0.3       | 0.25     | 3             | 0.8278                   | 0.3350                    | 0.2911                    |
| 8   | 0.5       | 0        | 3             | 0.7621                   | 0.1975                    | 0.1590                    |
| 8   | 0.5       | 0.0625   | 3             | 0.7769                   | 0.2254                    | 0.1976                    |
| 8   | 0.5       | 0.125    | 3             | 0.7929                   | 0.2567                    | 0.2328                    |
| 8   | 0.5       | 0.1875   | 3             | 0.8085                   | 0.2896                    | 0.2677                    |
| 8   | 0.5       | 0.25     | 3             | 0.8256                   | 0.3288                    | 0.2972                    |
| 12  | 0.3       | 0        | 3             | 0.7586                   | 0.1983                    | 0.1552                    |
| 12  | 0.3       | 0        | 2             | 0.6507                   | 0.2822                    | 0.2271                    |
| 12  | 0.3       | 0        | 1             | 0.5150                   | 0.3782                    | 0.3228                    |
| 12  | 0.3       | 0        | -1            | 0.2951                   | 0.5220                    | 0.4843                    |
| 12  | 0.3       | 0        | -2            | 0.2177                   | 0.5768                    | 0.5388                    |
| 12  | 0.5       | 0        | 3             | 0.7571                   | 0.1983                    | 0.1568                    |
| 12  | 0.5       | 0        | 2             | 0.6479                   | 0.2820                    | 0.2302                    |
| 12  | 0.5       | 0        | 1             | 0.5100                   | 0.3761                    | 0.3294                    |
| 12  | 0.5       | 0        | -1            | 0.2879                   | 0.5212                    | 0.4925                    |
| 12  | 0.5       | 0        | -2            | 0.2117                   | 0.5718                    | 0.5481                    |
| 12  | 0.3       | 0.125    | 3             | 0.7899                   | 0.2587                    | 0.2245                    |
| 12  | 0.3       | 0.125    | 2             | 0.6851                   | 0.3343                    | 0.2975                    |
| 12  | 0.3       | 0.125    | 1             | 0.5606                   | 0.4239                    | 0.3845                    |
| 12  | 0.3       | 0.125    | -1            | 0.3341                   | 0.5680                    | 0.5530                    |
| 12  | 0.3       | 0.125    | -2            | 0.2480                   | 0.6266                    | 0.6149                    |
| 12  | 0.5       | 0.125    | 3             | 0.7871                   | 0.2559                    | 0.2291                    |
| 12  | 0.5       | 0.125    | 2             | 0.6827                   | 0.3324                    | 0.3012                    |
| 12  | 0.5       | 0.125    | 1             | 0.5548                   | 0.4222                    | 0.3918                    |
| 12  | 0.5       | 0.125    | -1            | 0.3296                   | 0.5554                    | 0.5647                    |
| 12  | 0.5       | 0.125    | -2            | 0.2422                   | 0.6112                    | 0.6297                    |

TABLE IV: Charge densities on Cu and O sites for the same parameters as Table II.

| $L$ | $t'_{pp}$ | $\Delta_{dp}$ | $\langle n_{Cu} \rangle$ | $\langle n_{O_R} \rangle$ | $\langle n_{O_L} \rangle$ |
|-----|-----------|---------------|--------------------------|---------------------------|---------------------------|
| 8   | 0.3       | 3             | 0.8332                   | 0.2076                    | 0.1881                    |
| 8   | 0.3       | 2             | 0.7290                   | 0.2807                    | 0.2556                    |
| 8   | 0.3       | 1             | 0.6011                   | 0.3659                    | 0.3410                    |
| 8   | 0.3       | -1            | 0.3323                   | 0.6456                    | 0.4699                    |
| 8   | 0.3       | -2            | 0.2392                   | 0.7125                    | 0.5296                    |
| 16  | 0.3       | 3             | 0.8320                   | 0.2077                    | 0.1891                    |
| 16  | 0.3       | 2             | 0.7275                   | 0.2808                    | 0.2571                    |
| 16  | 0.3       | 1             | 0.5992                   | 0.3664                    | 0.3426                    |
| 16  | 0.3       | -1            | 0.3365                   | 0.5860                    | 0.4955                    |
| 16  | 0.3       | -2            | 0.2431                   | 0.6474                    | 0.5582                    |
| 24  | 0.3       | 3             | 0.8320                   | 0.2192                    | 0.1834                    |
| 24  | 0.3       | 2             | 0.7274                   | 0.2980                    | 0.2487                    |
| 24  | 0.3       | 1             | 0.5991                   | 0.3918                    | 0.3300                    |
| 24  | 0.3       | -1            | 0.3318                   | 0.6012                    | 0.4926                    |
| 24  | 0.3       | -2            | 0.2386                   | 0.6604                    | 0.5562                    |
| 8   | 0.5       | 3             | 0.8301                   | 0.2069                    | 0.1915                    |
| 8   | 0.5       | 2             | 0.7243                   | 0.2786                    | 0.2614                    |
| 8   | 0.5       | 1             | 0.5950                   | 0.3601                    | 0.3499                    |
| 8   | 0.5       | -1            | 0.3167                   | 0.4982                    | 0.5592                    |
| 8   | 0.5       | -2            | 0.2273                   | 0.5425                    | 0.6264                    |
| 16  | 0.5       | 3             | 0.8286                   | 0.2072                    | 0.1928                    |
| 16  | 0.5       | 2             | 0.7225                   | 0.2792                    | 0.2629                    |
| 16  | 0.5       | 1             | 0.5930                   | 0.3623                    | 0.3508                    |
| 16  | 0.5       | -1            | 0.3132                   | 0.5500                    | 0.5367                    |
| 16  | 0.5       | -2            | 0.2233                   | 0.5928                    | 0.6052                    |
| 24  | 0.5       | 3             | 0.8284                   | 0.2073                    | 0.1929                    |
| 24  | 0.5       | 2             | 0.7222                   | 0.2794                    | 0.2631                    |
| 24  | 0.5       | 1             | 0.5872                   | 0.3859                    | 0.3449                    |
| 24  | 0.5       | -1            | 0.3207                   | 0.5410                    | 0.5338                    |
| 24  | 0.5       | -2            | 0.2236                   | 0.5904                    | 0.6062                    |

## S.5. VALENCE TRANSITION APPROACH

### S.5.1. Negative charge-transfer gap and cation ionization energy, a consistent pattern

Theories of transition metal compounds, especially oxides, usually assume that the ligand anions are overwhelmingly closed shell in the undoped state ( $O^{2-}$  in oxides) and only a few of the anions are charged in the doped state ( $O^{1-}$ ). The concept of negative charge-transfer gap, that the energy of charge-transfer from ligand to metal can be negative, and that even in the undoped state anions can be overwhelmingly open shell, is antithetical to this traditional idea even though this possibility was discussed in the classic paper by Zaanen, Sawatzky and Allen [S3]. Computational work that have found negative charge-transfer gap in different systems [S4–8] are based on many-body corrections to band theoretical approaches (LSDA +  $U$ , DFT + DMFT). The theories correctly emphasize that the primary requirements for negative charge-transfer gap are that the formal oxidation state of the transition metal cation must be large, and covalency effects are strong relative to the charge-transfer gap. Our approach to negative charge-transfer agrees with these requirements, but goes a step further by pointing out a common characteristic shared by the metal cation in nearly all negative charge-transfer compounds, viz., the cation in the lower charged-state is either exactly closed shell or exactly half-filled once crystal structure effects are taken into consideration [S9]. These are precisely when ionization to the next higher charged states can be energetically expensive. In Fig. S6(a) we have reproduced our previous plot of the 4th ionization energies of Pb, Bi and Po, neighboring elements in the Periodic Table. The closed-shell electron configuration of  $Bi^{3+}$  is behind its relatively high ionization energy. Fig. S6(b) shows a similar plot for the 4th ionization energy of  $3d$  transition elements. The local peak at  $Fe^{3+}$  is due to its half-filled  $d^5$  electron occupancy. Negative charge-transfer gaps in  $BaBiO_3$  [S8] and  $FeO_2$  [S5,6] are ascribed to these higher-than-usual ionization energies in the state with the lower cation charge.

For  $d$ -electron occupancies less than 5 crystal structure effects become relevant. For  $CrO_2$ , as was noted correctly by Korotin *et al.* [S4], formal oxidation state of  $Cr^{4+}$  with 2 electrons occupying two of the  $t_{2g}$  orbitals would have led to Mott insulating behavior. Based on LSDA +  $U$  calculations the authors found nearly pure  $2p$  electrons from the oxygen anions to cross the Fermi level in this material, with  $d-d$  Coulomb repulsion playing a minimal role. This is also anticipated within our ionic model, within which with octahedral anion arrangement the  $Cr^{3+}$  electron configuration is half-filled and therefore very stable, and the overall oxygen charge is  $-1.5$ , exactly what is found [S6] in  $FeO_2$ . Finally the stability of closed-shell  $Au^{1+}$  explains the negative charge-transfer in  $AuTe_2$  [S7]. There exists then a consistent pattern among most negative charge-transfer compounds.

In Fig. S6(c) we show the behavior of the second ionization energies of  $3d$  transition elements. The large ionization energy of  $Cu^{1+}$ , relative to its neighbors  $Ni^{1+}$  and  $Zn^{2+}$ , is once again due to its closed-shell  $d^{10}$  configuration. Based on the behavioral pattern pointed out above, it is natural to surmise that cuprates are very close to the positive-negative charge-transfer boundary (Eq. 2 of text). Doping or pressure-induced transition to the closed-shell stable lower valent state here is analogous to the metallicity-driven self-doped negative charge-transfer gap in  $CrO_2$  [S4].

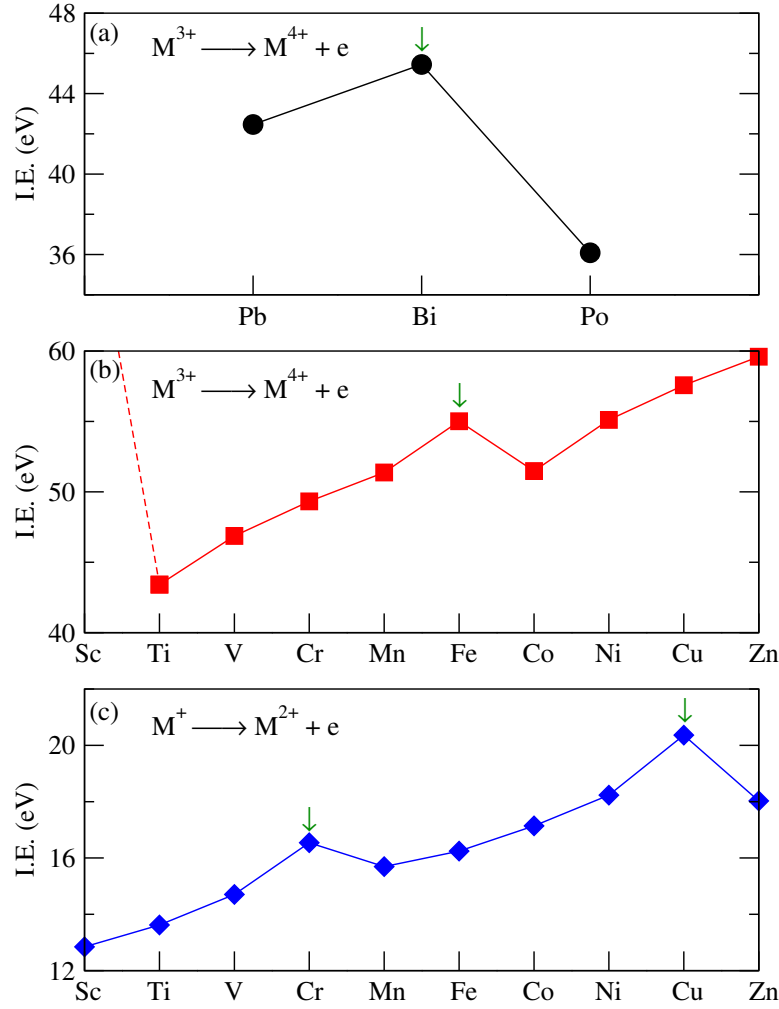

FIG. S6: (a) Fourth ionization energies of Pb, Bi, and Po. (b) Fourth and (c) second ionization energies of 3d transition metals. Note the peaks at  $\text{Bi}^{3+}$ ,  $\text{Fe}^{3+}$  and  $\text{Cu}^{1+}$ .

### S.5.2. Charge on ladder layer O-anions, post-valence transition

In what follows we make no distinction between  $\text{Sr}^{2+}$  and  $\text{Ca}^{2+}$ , as we are interested in counting charges only. We begin by assuming that 7 of 14  $\text{Sr}^{2+}$ -ions per formula unit of SCCO are “associated” with the ladder layer. The corresponding ladder formula unit is written as  $\text{Sr}_7\text{Cu}_{14}\text{O}_{21}$ . If all Cu-ions have charge +2, that leaves no extra holes on the ladder layer and all 6 holes per formula unit would be occupying the chain layer, which we know is incorrect. It is nevertheless instructive to calculate the charges on the Cu and O-ions following valence transition starting from this limit. Valence transition that takes Cu-ion charge from +2.0 to +1.0 would make the charge on O-ions  $-1.33$ . Assuming that the charges on the Cu-ions are not precisely integral, the O-ion charges are  $-1.47$  for realistic Cu-ion charge of +1.2.

One can now repeat the above estimations with the assumption of chemical formula units  $\text{Sr}_6\text{Cu}_{14}\text{O}_{21}$  (corresponding to 2 holes on the ladder layer and 4 on the chain layer before the valence transition). For Cu-ion charge of +1.2 we now will have average charge of  $-1.37$  on the oxygens. Similarly, with 1 additional hole in the ladder layer before valence transition the O-anion charge following valence transition is  $-1.42$ . In all cases it is close to the  $-1.5$  estimated by the author of reference S5, and also close to the required for electron correlation-driven SC (see main text, especially references 43 and 44).

### S.5.3. Pressure-driven valence transition

Bond orders and their ratios, for the same parameters as in Fig. 3 of main text, with however  $t'_{pp} = 0.3$ .

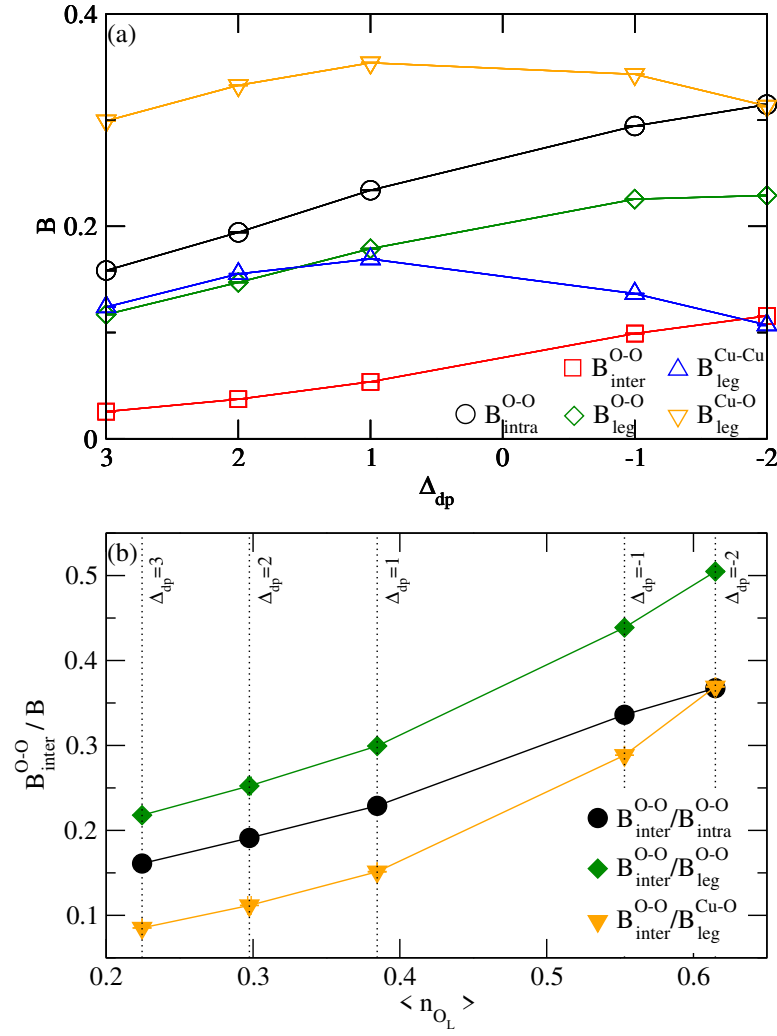

FIG. S7: (a) Bare bond orders and (b) their ratio for  $t'_{pp} = 0.3$  for the same parameters as Fig. 3 in the main text.

- 
- [S1] Matthew Fishman, Steven R. White, and E. Miles Stoudenmire. The ITensor software library for tensor network calculations. <https://arxiv.org/abs/2007.14822>, 2020.
- [S2] E. M. Stoudenmire and S. R. White. Real-space parallel density matrix renormalization group. *Phys. Rev. B*, 87:155137, 2013.
- [S3] J. Zaanen, G. A. Sawatzky, and J. W. Allen. Band gaps and electronic structure of transition-metal compounds. *Phys. Rev. Lett.*, 55:418–421, 1985.
- [S4] A. Korotin, V. I. Anisimov, D. I. Khomskii, and G. A. Sawatzky.  $\text{CrO}_2$ : a self-doped double exchange ferromagnet. *Phys. Rev. Lett.*, 80:4305–4308, 1998.
- [S5] S. S. Streltsov, A. O. Shorikov, S. L. Skornyakov, A. I. Poteryaev, and D. I. Khomskii. Unexpected 3+ valence of iron in  $\text{FeO}_2$ , a geologically important material lying “in between” oxides and peroxides. *Sci. Rep.*, 7:13005, 2017.
- [S6] E. Koemets et al. Revealing the complex nature of bonding in the binary high-pressure compound  $\text{FeO}_2$ . *Phys. Rev. Lett.*, 126:106001, 2021.
- [S7] S. V. Streltsov, V. V. Roizenc, A. V. Ushakova, A. R. Oganov, and D. I. Khomskii. Old puzzle of incommensurate crystal structure of calaverite  $\text{AuTe}_2$  and predicted stability of novel  $\text{AuTe}$  compound. *Proc. Natl. Acad. Sci. USA*, 115:9945–9950, 2018.
- [S8] A. Khazraie, K. Foyevtsova, I. Elfimov, and G. A. Sawatzky. Oxygen holes and hybridization in the bismuthates. *Phys. Rev. B*, 97:075103, 2018.
- [S9] S. Mazumdar. Negative charge-transfer gap and even parity superconductivity in  $\text{Sr}_2\text{RuO}_4$ . *Phys. Rev. Res.*, 2:023382, 2020.
